# Supplementary material for: HandyPriors: Physically Consistent Perception of Hand-Object Interactions with Differentiable Priors
Source: arXiv:2311.16552 source file (2023-12-26)
Supplement: Supplementary file 1 [file appendix.tex]

\section{Extended Kalman Filter}
\label{app:ekf}

We have a dynamic system,
\begin{equation}
    \xx_t=f(\xx_{t-1}, \uu_t) + \epsilon_{s},
    \zz_t=h(\xx_t)+\epsilon_{o},
\end{equation}
where $\xx$ is the state, $\uu$ is the control, $\zz$ is the observation, $\epsilon_{s}$ and $\epsilon_{o}$ are multivariate Gaussian noises with covariance $\QQ$ and $\RR$ respectively, $f(\cdot),h(\cdot)$ are \textit{differentiable} functions for states and observation, respectively. EKF can predict the state $\hat{\xx}_{t}$ and covariance matrix $\PP_t$ given the observation $\zz$. The EKF works in the following steps for each frame,
\begin{align}
    \FF &= \partial f/\partial \hat{\xx}_{t-1}\\ 
    \xx'&=f(\hat{\xx}_{t-1}, \uu_t)\\
    \HH &= \partial h/\partial\xx'\\
    \PP'&=\FF_t\PP_{t-1}\FF_t\trans+\QQ\\
    \yy&=\zz_t-h(\xx')\\
    \mathbf{S}&=\HH\PP'\HH\trans+\RR\\
    \KK&=\PP'\HH\trans\mathbf{S}^{-1}\\
    \hat{\xx}_{t}&=\xx'+\KK\yy\\
    \hat{\PP}_t&=(\II-\KK\HH)\PP'
\end{align}

More detailed derivation can be found in ~\cite{ribeiro2004kalman}. In our experiments, we use the 3D positions of fingertips as the control input. The observation signal could be the hand pose, object bounding boxes, etc.

\section{Quasistatic Time-stepping}
\label{app:timestepping}
We assume that the relative sliding of the contact points on the object is small. For simplicity, we approximately treat the fingertips as the contact points $\vv$. Since the object is rigid, we could treat the point cloud at two adjacent frames under rigid transformation. Therefore, we could use SVD-based rigid point registration~\cite{sorkine2017least} to compute the relative rotation and translation.

\section{Contact Refinement}
Table~\ref{tab:contact} show the quantitative comparisons with ContactOpt. It demonstrates that the two methods have comparable performance on the 3D hand and object errors.
\label{app:contact}
\begin{table}[]
    \centering
    \caption{\textbf{Error after contact-based pose refinement.} Our differentiable contact module is used to refine the pose given the contact status and achieves comparable results as ContactOpt~\cite{grady2021contactopt}.}
    \begin{tabular}{@{}lccc@{}}
    \toprule
    Method      & \multicolumn{1}{l}{hand joints} & \multicolumn{1}{l}{hand verts} & \multicolumn{1}{l}{object verts} \\
    \midrule
    ContactOpt & 0.0143   & 0.0137  & 0.0367  \\
    ours        & 0.0143   & 0.0136  & 0.0364 \\
    \bottomrule
    \end{tabular}
    \label{tab:contact}
\end{table}

\section{Implementation Details}
Our differentiable priors are implemented using Pytorch and optimized by Stochastic Gradient Descent (SGD) with learning rate 0.01. The weights of loss terms are $\{\lambda_i\}{i=1,..,6}=\{0.1, 0.3, 0.005, 0.001, 1, 0.1\}$. The profiling numbers
 in Table~\ref{tab:ablation} are obtained on a desktop with an Intel(R) Xeon(R) W-2123 CPU @ 3.60GHz and an NVIDIA Titan XP GPU. The EKF is from the torchfilter~\cite{lee2020multimodal} and the differentiable renderer is SoftRas~\cite{liu2019softras}.

\section{More Visual Results}
Please kindly refer to our supplementary video for more visual results.
